# Supplementary material for: Privacy Preserving Spam Filtering
Source: arXiv:1102.4021 source file (2011-09-18)
Supplement: Supplementary file 1 [file appendix.tex]

Graphical description of the protocol.

\begin{center}
  \begin{tabular}{ c c c }
    \textbf{Alice} & & \textbf{Bob} \\
    $E[y_iw_{(t)}^Tx_i]$ & $\xleftarrow[O(d)]{E[w_{(t)}]}$ & $w_{(t)}$ \\~\\
    gen $r_i$  & $\xrightarrow[O(n)]{E[y_iw_{(t)}^Tx_i - r_i]}$ & $y_iw_{(t)}^Tx_i - r_i$ \\~\\
    $E\left[e^{y_iw_{(t)}^Tx_i}\right]$ & $\xleftarrow[O(d)]{E\left[e^{y_iw_{(t)}^Tx_i - r_i}\right]}$ & $e^{y_iw_{(t)}^Tx_i - r_i}$ \\
    $E[1+e^{y_iw_{(t)}^Tx_i }]$ &  &  \\~\\
    gen $q_i$ & $\xrightarrow[O(n)]{E\left[q_i\left(1+e^{y_iw_{(t)}^Tx_i }\right)\right]}$ &  $q_i\left(1+e^{y_iw_{(t)}^Tx_i }\right)$ \\~\\
    $E\left[\frac{1}{1+e^{y_i w_{(t)}^T x_i}}\right]$ 
    & $\xleftarrow[O(n)]{E\left[\frac{1}{q_i\left(1+e^{y_i w_{(t)}^T x_i}\right)}\right]}$ 
    & $\frac{1}{q_i\left(1+e^{y_i w_{(t)}^T x_i}\right)}$ \\~\\
    $E\left[\frac{y_ix_i^T}{1+e^{y_iw_{(t)}^Tx_i }}\right]$ 
    & $\xrightarrow[O(d)]{E\left[\sum_i \frac{y_ix_i^T}{1+e^{y_iw_{(t)}^Tx_i }}\right]}$ & $\nabla \ell(w,x,y)$
  \end{tabular}
\end{center}
